# Supplementary material for: Continuous Cost Aggregation for Dual-Pixel Disparity Extraction
Source: arXiv:2306.07921 source file (2023-06-13)
Supplement: Supplementary file 1 [file STEREO_supp_res.tex]

\begin{figure*}[t]
  \begin{center}
   \begin{tabular}{c@{\hspace{1mm}}c@{\hspace{1mm}}c@{\hspace{1mm}}c@{\hspace{1mm}}c@{\hspace{1mm}}c}

      \includegraphics[width=0.15\linewidth]{\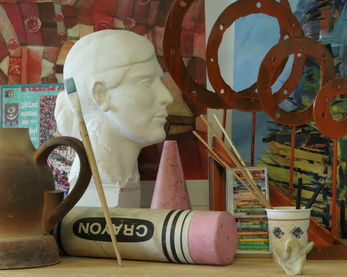} &
      \includegraphics[width=0.15\linewidth]{\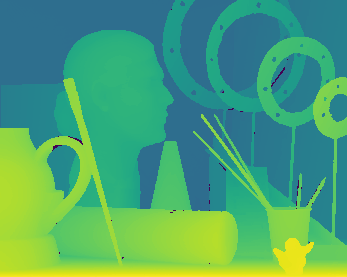} &
      \includegraphics[width=0.15\linewidth]{\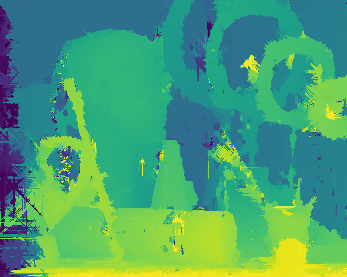} &
      \includegraphics[width=0.15\linewidth]{\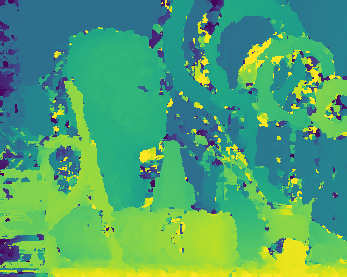} &
      \includegraphics[width=0.15\linewidth]{\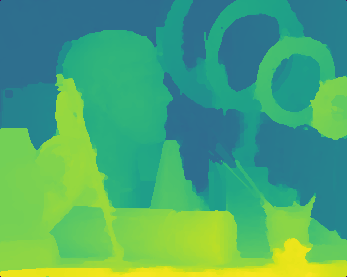} &
      \includegraphics[width=0.15\linewidth]{\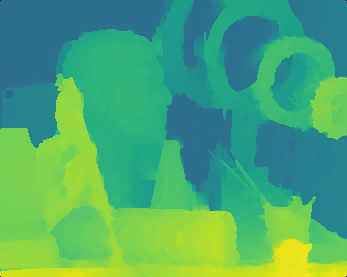} \\

      \includegraphics[width=0.15\linewidth]{\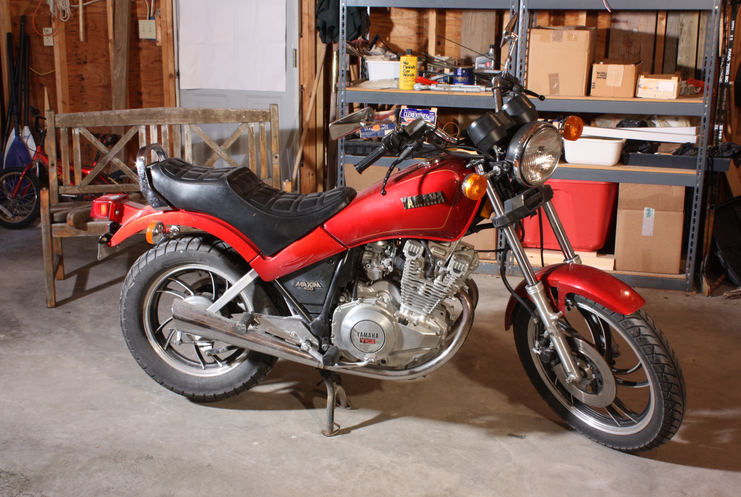} &
      \includegraphics[width=0.15\linewidth]{\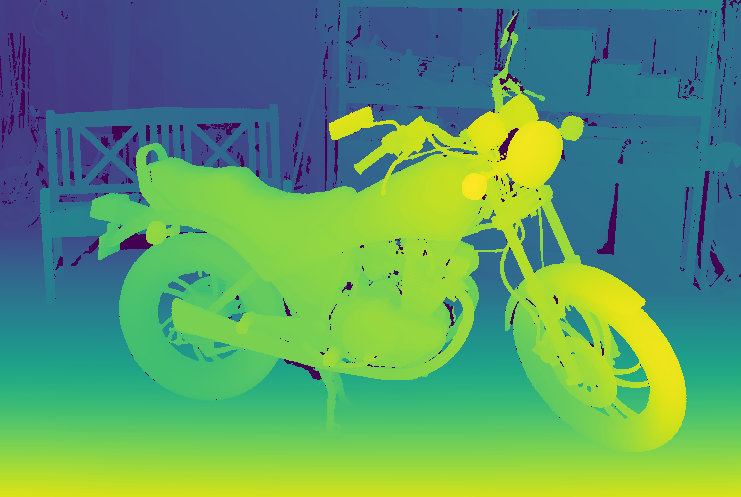} &
      \includegraphics[width=0.15\linewidth]{\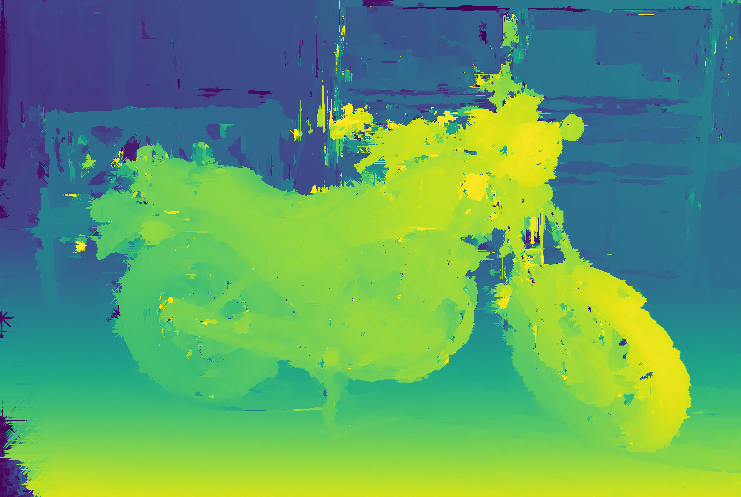} &
      \includegraphics[width=0.15\linewidth]{\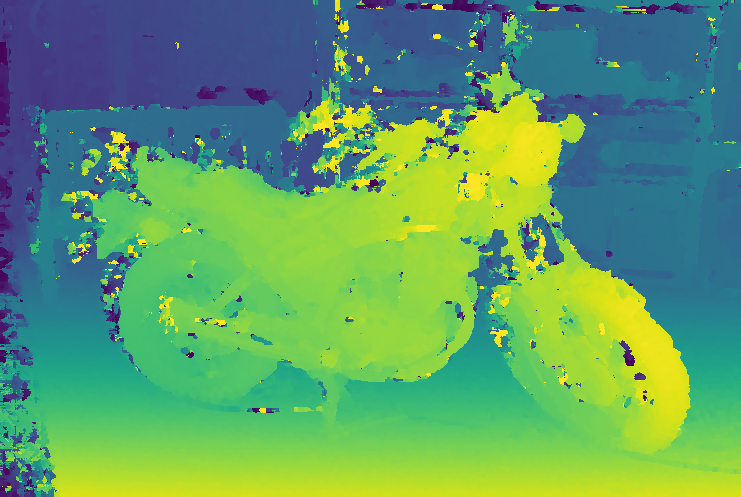} &
      \includegraphics[width=0.15\linewidth]{\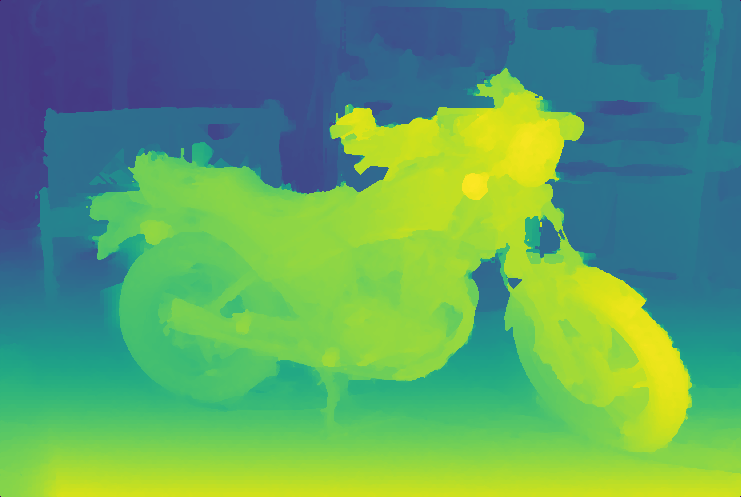} &
      \includegraphics[width=0.15\linewidth]{\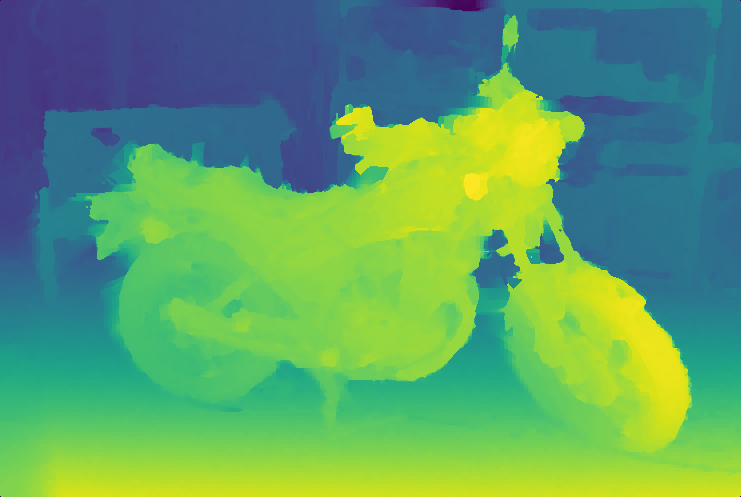} \\

      \includegraphics[width=0.15\linewidth]{\Figs/Stereo_CSGM_vs_SGM/images/im_12.png} &
      \includegraphics[width=0.15\linewidth]{\Figs/Stereo_CSGM_vs_SGM/GT/GT12.png} &
      \includegraphics[width=0.15\linewidth]{\Figs/Stereo_CSGM_vs_SGM/csgm_no_filter_no_mask/CSGM_no_filter12.png} &
      \includegraphics[width=0.15\linewidth]{\Figs/Stereo_CSGM_vs_SGM/sgm_no_filter_no_mask/SGM_no_filter12.png} &
      \includegraphics[width=0.15\linewidth]{\Figs/Stereo_CSGM_vs_SGM/csgm_filter_no_mask/CSGM12.png} &
      \includegraphics[width=0.15\linewidth]{\Figs/Stereo_CSGM_vs_SGM/sgm_filter_no_mask/SGM12.png} \\
      
    %   \includegraphics[width=0.15\linewidth]{\Figs/Stereo_CSGM_vs_SGM/images/im_11.png} &
    %   \includegraphics[width=0.15\linewidth]{\Figs/Stereo_CSGM_vs_SGM/GT/GT11.png} &
    %   \includegraphics[width=0.15\linewidth]{\Figs/Stereo_CSGM_vs_SGM/csgm_no_filter_no_mask/CSGM_no_filter11.png} &
    %   \includegraphics[width=0.15\linewidth]{\Figs/Stereo_CSGM_vs_SGM/sgm_no_filter_no_mask/SGM_no_filter11.png} &
    %   \includegraphics[width=0.15\linewidth]{\Figs/Stereo_CSGM_vs_SGM/csgm_filter_no_mask/CSGM11.png} &
    %   \includegraphics[width=0.15\linewidth]{\Figs/Stereo_CSGM_vs_SGM/sgm_filter_no_mask/SGM11.png} \\ 
      
    %   \includegraphics[width=0.15\linewidth]{\Figs/Stereo_CSGM_vs_SGM/images/im_11.png} &
    %   \includegraphics[width=0.15\linewidth]{\Figs/Stereo_CSGM_vs_SGM/GT/GT11.png} &
    %   % \includegraphics[width=0.15\linewidth]{\Figs/Stereo_CSGM_vs_SGM/csgm_no_filter_no_mask/CSGM_no_filter11.png} &
    %   % \includegraphics[width=0.15\linewidth]{\Figs/Stereo_CSGM_vs_SGM/sgm_no_filter_no_mask/SGM_no_filter11.png} &
    %   \includegraphics[width=0.15\linewidth]{\Figs/Stereo_CSGM_vs_SGM/csgm_filter_no_mask/CSGM11.png} &
    %   \includegraphics[width=0.15\linewidth]{\Figs/Stereo_CSGM_vs_SGM/sgm_filter_no_mask/SGM11.png} &
    %   \includegraphics[width=0.15\linewidth]{\Figs/Stereo_CSGM_vs_SGM/mask_CSGM/CSGM_mask_1pix11.png} &
    %   \includegraphics[width=0.15\linewidth]{\Figs/Stereo_CSGM_vs_SGM/mask_SGM/SGM_mask_1pix11.png} \\

      (a) Image & (b) GT & (c) CCA  & (d) SGM  & (e) CCA + filter & (f) SGM + filter
    \end{tabular}
    \end{center}
 \caption{Additional results on middlebury training dataset at quarter resolution, showing our algorithm performs similar to SGM.} %\Monin{I removed the image} \sagi{In the last row, the floor results for the CSGM is very noisy. It shouldn't be like that and indicates an issue. Our main point was that we produce smooth sub-pixel results, but it looks noisier compared to SGM} \Monin{This is an area with a lot of repeated texture - so the algorithm doesn't do as good as SGM (the entire floor is just repeated texture). Also the range of disparity is about 80 pixels, so noise is not sub-pixel smooth but points with high confidence and wrong integer disparity}}
 \label{fig:Stereo_result_supp}
\end{figure*}
